# Supplementary material for: BSODiag: A Global Diagnosis Framework for Batch Servers Outage in Large-scale Cloud Infrastructure Systems
Source: arXiv:2502.15728 source file (2025-01-31)
Supplement: Supplementary file 1 [file appendix.tex]

\section{APPENDIX}
